# Supplementary material for: Adapting Physics-Informed Neural Networks to Improve ODE Optimization in Mosquito Population Dynamics
Source: arXiv:2406.05108 source file (2025-01-29)
Supplement: Supplementary file 1 [file S1_Appendix.tex]

\begin{document}
\title Supporting Information
\end{document}
